# Supplementary material for: Vacancy-stabilized crystalline order in hard cubes
Source: arXiv:1111.3466 ancillary file (2012-09-16)
Supplement: Supplementary file 1 [file cubesSI.pdf]

# Vacancy-stabilized crystalline order in hard cubes: Supporting Information

Frank Smallenburg, Laura Filion, Matthieu Marechal, and Marjolein Dijkstra

## SIMULATION TECHNIQUES

We study perfectly sharp hard cubes with edge length $\sigma$, using both Monte Carlo (MC) and event-driven molecular dynamics (EDMD) simulations. In both types of simulation, overlaps are detected using an algorithm based on the separating axis theorem.[1] According to this theorem, for any two non-overlapping convex bodies there exists an axis onto which both shapes can be projected without overlapping. In other words, if both shapes are projected onto this separating axis, the resulting two intervals on the axis are disjoint. No such axis exists if the particles overlap. For two convex polyhedral particles, only a finite number of possible separating axes need to be checked: the potential separating axes are either parallel to a normal of one of the faces of either of the two particles, or perpendicular to the plane spanned by one of the edges of the first particle and one of the edges of the second particle. If none of these directions correspond to a separating axis, the particles overlap.

For a cube-shaped particle $a$, all face normals and edges are parallel to one of the three perpendicular axes $\mathbf{u}_{a,i}$ of unit length, with $i \in \{1, 2, 3\}$. Thus, the fifteen potential separating axes for two cubes are given by $\mathbf{u}_{a,i}$, $\mathbf{u}_{b,i}$, and $\mathbf{u}_{a,i} \times \mathbf{u}_{b,j}$. To calculate the projection of both particles onto a potential separating axis $\mathbf{L}$, it is convenient to take the center $\mathbf{r}_a$ of particle $a$ as the origin, and placing particle $b$ at position $\mathbf{d} = \mathbf{r}_b - \mathbf{r}_a$. Since the particles are convex, it is sufficient to project the vertices of each particle onto $\mathbf{L}$. For particle $a$, the positions of the vertices are given by $(\pm\mathbf{u}_{a,1} \pm \mathbf{u}_{a,2} \pm \mathbf{u}_{a,3})\sigma/2$. The projections onto $\mathbf{L}$ are thus contained in the interval $[-R_a(\mathbf{L}), R_a(\mathbf{L})]$, with

$$R_a(\mathbf{L}) = \frac{\sigma}{2} \sum_{i=1}^{3} |\mathbf{u}_{a,i} \cdot \mathbf{L}| . \tag{1}$$

Here, we have taken the separating axis $\mathbf{L}$ to be of unit length. Similarly, the projections of the vertices of particle $b$ are in an interval centered around $\mathbf{d} \cdot \mathbf{L}$ with radius

$$R_b(\mathbf{L}) = \frac{\sigma}{2} \sum_{i=1}^{3} |\mathbf{u}_{b,i} \cdot \mathbf{L}| . \tag{2}$$

If $\mathbf{L}$ is a separating axis, these intervals are non-overlapping. In that case,

$$\mathbf{d} \cdot \mathbf{L} > R_a(\mathbf{L}) + R_b(\mathbf{L}). \tag{3}$$

If this inequality holds for any one of the potential separating axes, the two particles do not overlap. We can use Eq. 3 to design a distance function $f$ for two particles:

$$f(a, b) = \max_{\mathbf{L}} \left\{ \mathbf{d} \cdot \mathbf{L} - (R_a(\mathbf{L}) + R_b(\mathbf{L})) \right\}, \tag{4}$$

where the maximum is taken over all potential choices for $\mathbf{L}$. The function $f(a, b)$ is negative whenever the particles $a$ and $b$ overlap, and positive when they do not. Additionally, $f$ is continuous as a function of translations and rotations of either particle. To predict collisions in the EDMD simulations, we use numerical root-finding algorithms to find the roots of $f$ as a function of time, following the methods used in Ref. [2]. An Andersen thermostat was used to keep the temperature in the EDMD simulation fixed: at fixed time intervals, a random selection of particles are given a new velocity and angular velocity drawn from a Maxwell-Boltzmann distribution.[3] The standard unit of time in EDMD simulations is given by $\tau = \sqrt{\beta m \sigma^2}$, where $m$ is the mass of a cube, and $\beta = 1/k_B T$ with $k_B$ Boltzmann's constant and $T$ the temperature. The simulations of crystals with $N_L = 64000$ lattice sites were run for at least $500\tau$, after which no further changes to the lattice structure were observed. To determine the density profiles (Fig. 1) and the global positional order (Fig. 2) in these simulations, snapshots were taken every $8\tau$, and the $G_{\mathrm{global}}$ was calculated and averaged over the last 20 snapshots. To determine equations of state, simulations with $N_L = 8000$ or 9000 lattice sites were allowed to run for at least $2500\tau$, with simulations near the coexistence region being up to four times longer to compensate for longer correlation times in the system.

## DIRECT OBSERVATION OF FLUID-SOLID COEXISTENCE

We observed coexistence between the fluid and solid phase for packing fractions $0.455 \leq \eta \leq 0.485$ in EDMD simulations of $N = 64000$ particles starting from a defect-free simple cubic crystal state. Typical snapshots of resulting configurations are shown in Supporting Figure S1. The largest crystalline cluster in the system was found based on the local bond order parameter $q_4$ [4]. As the density increases, the shape of the interface goes through a series of stages [5]: a roughly spherical crystalline cluster in a majority disordered fluid phase ($\eta = 0.45$), a cylindrical crystalline cluster spanning the simulation box in one direction in a fluid phase ($\eta = 0.455$), two slab-like regions of fluid and solid separated by planar interfaces ($0.46 \leq \eta \leq 0.47$), and a majority crystal phase containing either a cylindrical fluid cluster ($0.475 \leq \eta \leq 0.48$), or small pockets of fluid in a crystal phase ($0.485 \leq \eta \leq 0.49$). This sequence of phase coexistence is typical of a first-order phase transition [5].

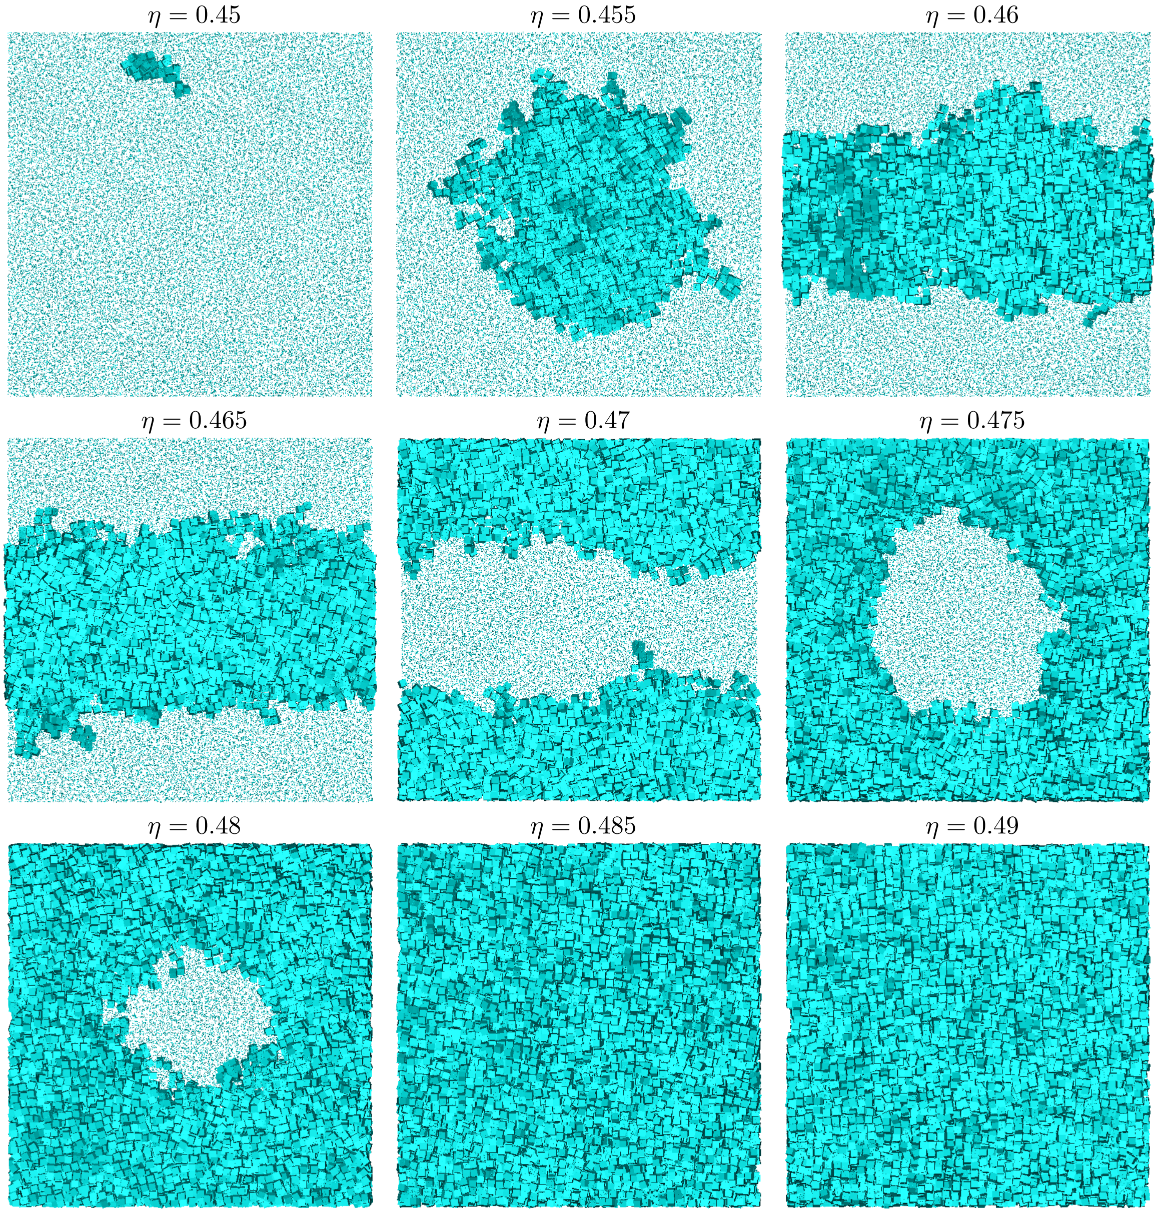


FIG. S1: Snapshots of EDMD simulations with $N = 64000$ hard cubes, at a range of packing fractions in the coexistence region. For each snapshot, clusters were determined based on $q_4$. Particles in the largest solid cluster are shown at actual size, while the other particles are displayed much smaller. Although the phase that coexists with the fluid for $\eta \leq 0.485$ looks disordered, it has at least local simple-cubic-like positional order, as indicated by the $q_4$ criterion. However, we cannot exclude that the positional order is only finite ranged, which would be indicative of a cubatic phase.

## SPONTANEOUS VACANCY FORMATION

As discussed in the main text, simulations of $N = 64000$ particles performed at packing fractions $\eta = 0.52 - 0.54$ and initialized with *no vacancies* displayed unusual behavior. In particular, in many cases, the underlying cubic lattice which started out commensurate with the simulation box rotated during the simulation. In the remaining cases, the system spontaneously increased the number of lattice sites. These two cases are shown in Supporting Figure S2.

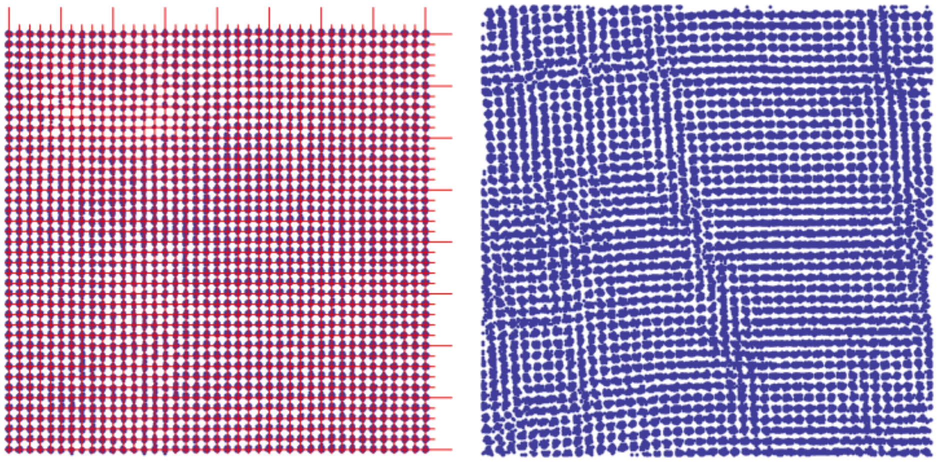

FIG. S2: Peaks in the 2D projection of the density profile in two simulations of hard cubes at packing fractions $\eta = 0.52$ (left) and $\eta = 0.525$ (right). For both simulations, the initial configuration was a simple cubic crystal of $N = 40^3$ particles and $N_L = 40^3$ lattice sites, i.e. no vacancies. However, the number of lattice sites was found to change spontaneously by either the addition of extra layers (left) or rotation of the crystal structure (right). The red lines in the picture on the left indicate the 41 evenly spaced layers in both directions.

## COMMON TANGENT CONSTRUCTION

The plot in Supporting Figure S3 shows the common tangent construction discussed in the main text. The solid line was obtained by minimizing the free energy with respect to the net vacancy concentration for a range of packing fractions, and by fitting the resulting data with a high-order polynomial. The fluid line is the result of a thermodynamic integration of the fluid equation of state.

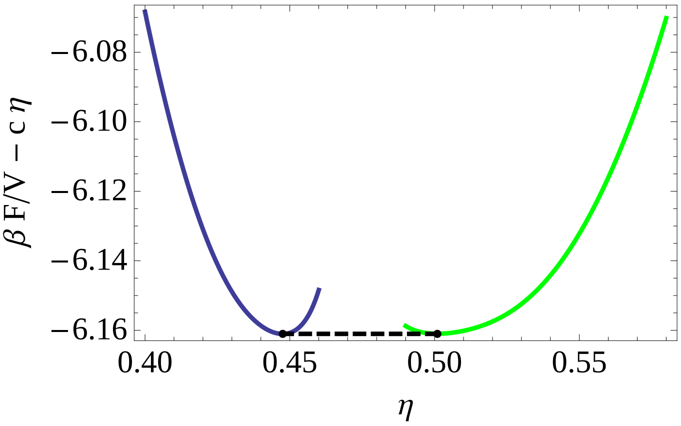


FIG. S3: The common tangent construction used to determine the bulk coexistence between the fluid and the solid phase in hard cubes. The plot shows the fluid free energy (left), solid free energy (right), and the common tangent (dashed line). Note that a linear function with a constant slope $c = 18.42$ has been subtracted for clarity. This does not influence the resulting coexistence.

## MEAN SQUARED DISPLACEMENT

Supporting Figure S4 shows the mean squared displacement as a function of time in the vacancy-rich crystal phase for packing fractions $\eta = 0.52$ and 0.56. The points are measured in EDMD simulations with $N_L = 8000$ particles, with the number of vacancies corresponding to the equilibrium concentration as determined from the free energy calculations.

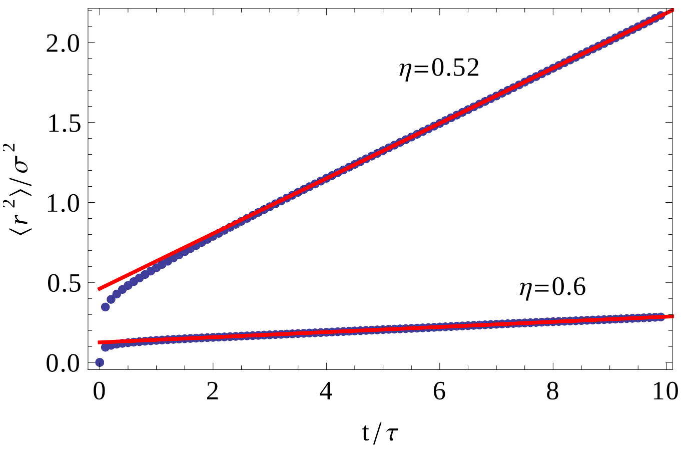


FIG. S4: Mean squared displacement as a function of time for two systems of cubes with $N_L = 8000$ lattice sites. The vacancy concentrations used for packing fraction $\eta = 0.52$ and 0.60 were $\alpha = 0.029$ and 0.0027, respectively. The lines are fits through the linear part of the data, with the slope proportional to the long-time self-diffusion constant


[1] S. Gottschalk, M. C. Lin, and D. Manocha, OBBTree: a hierarchical structure for rapid interference detection, *Proc. ACM SIGGRAPH*, 171 (1996).

[2] L. H. de la Peña, R. van Zon, J. Schofield and S. B. Opps, Discontinuous molecular dynamics for semiflexible and rigid bodies, *J. Chem. Phys.* 126:074105 (2007).

[3] D. Frenkel and B. Smit, Understanding Molecular Simulations: From Algorithms to Applications (Academic Press, London, UK, 2002).

[4] P. R. ten Wolde, M. J. Ruiz-Montero, and D. Frenkel, Numerical calculation of the rate of crystal nucleation in a Lennard-Jones system at moderate undercooling, *J. Chem. Phys.* 104:9932 (1996).

[5] M. Schrader, P. Virnau, and K. Binder, Simulation of vapor-liquid coexistence in finite volumes: A method to compute the surface free energy of droplets, *Phys. Rev. E* 79:061104 (2009).
